# Supplementary material for: Learning Task-General Representations with Generative Neuro-Symbolic Modeling
Source: arXiv:2006.14448 source file (2021-01-23)
Supplement: Supplementary file 1 [file marginals_theory.tex]

\begin{figure}[ht]
    \centering
    \includegraphics[width=\hsize]{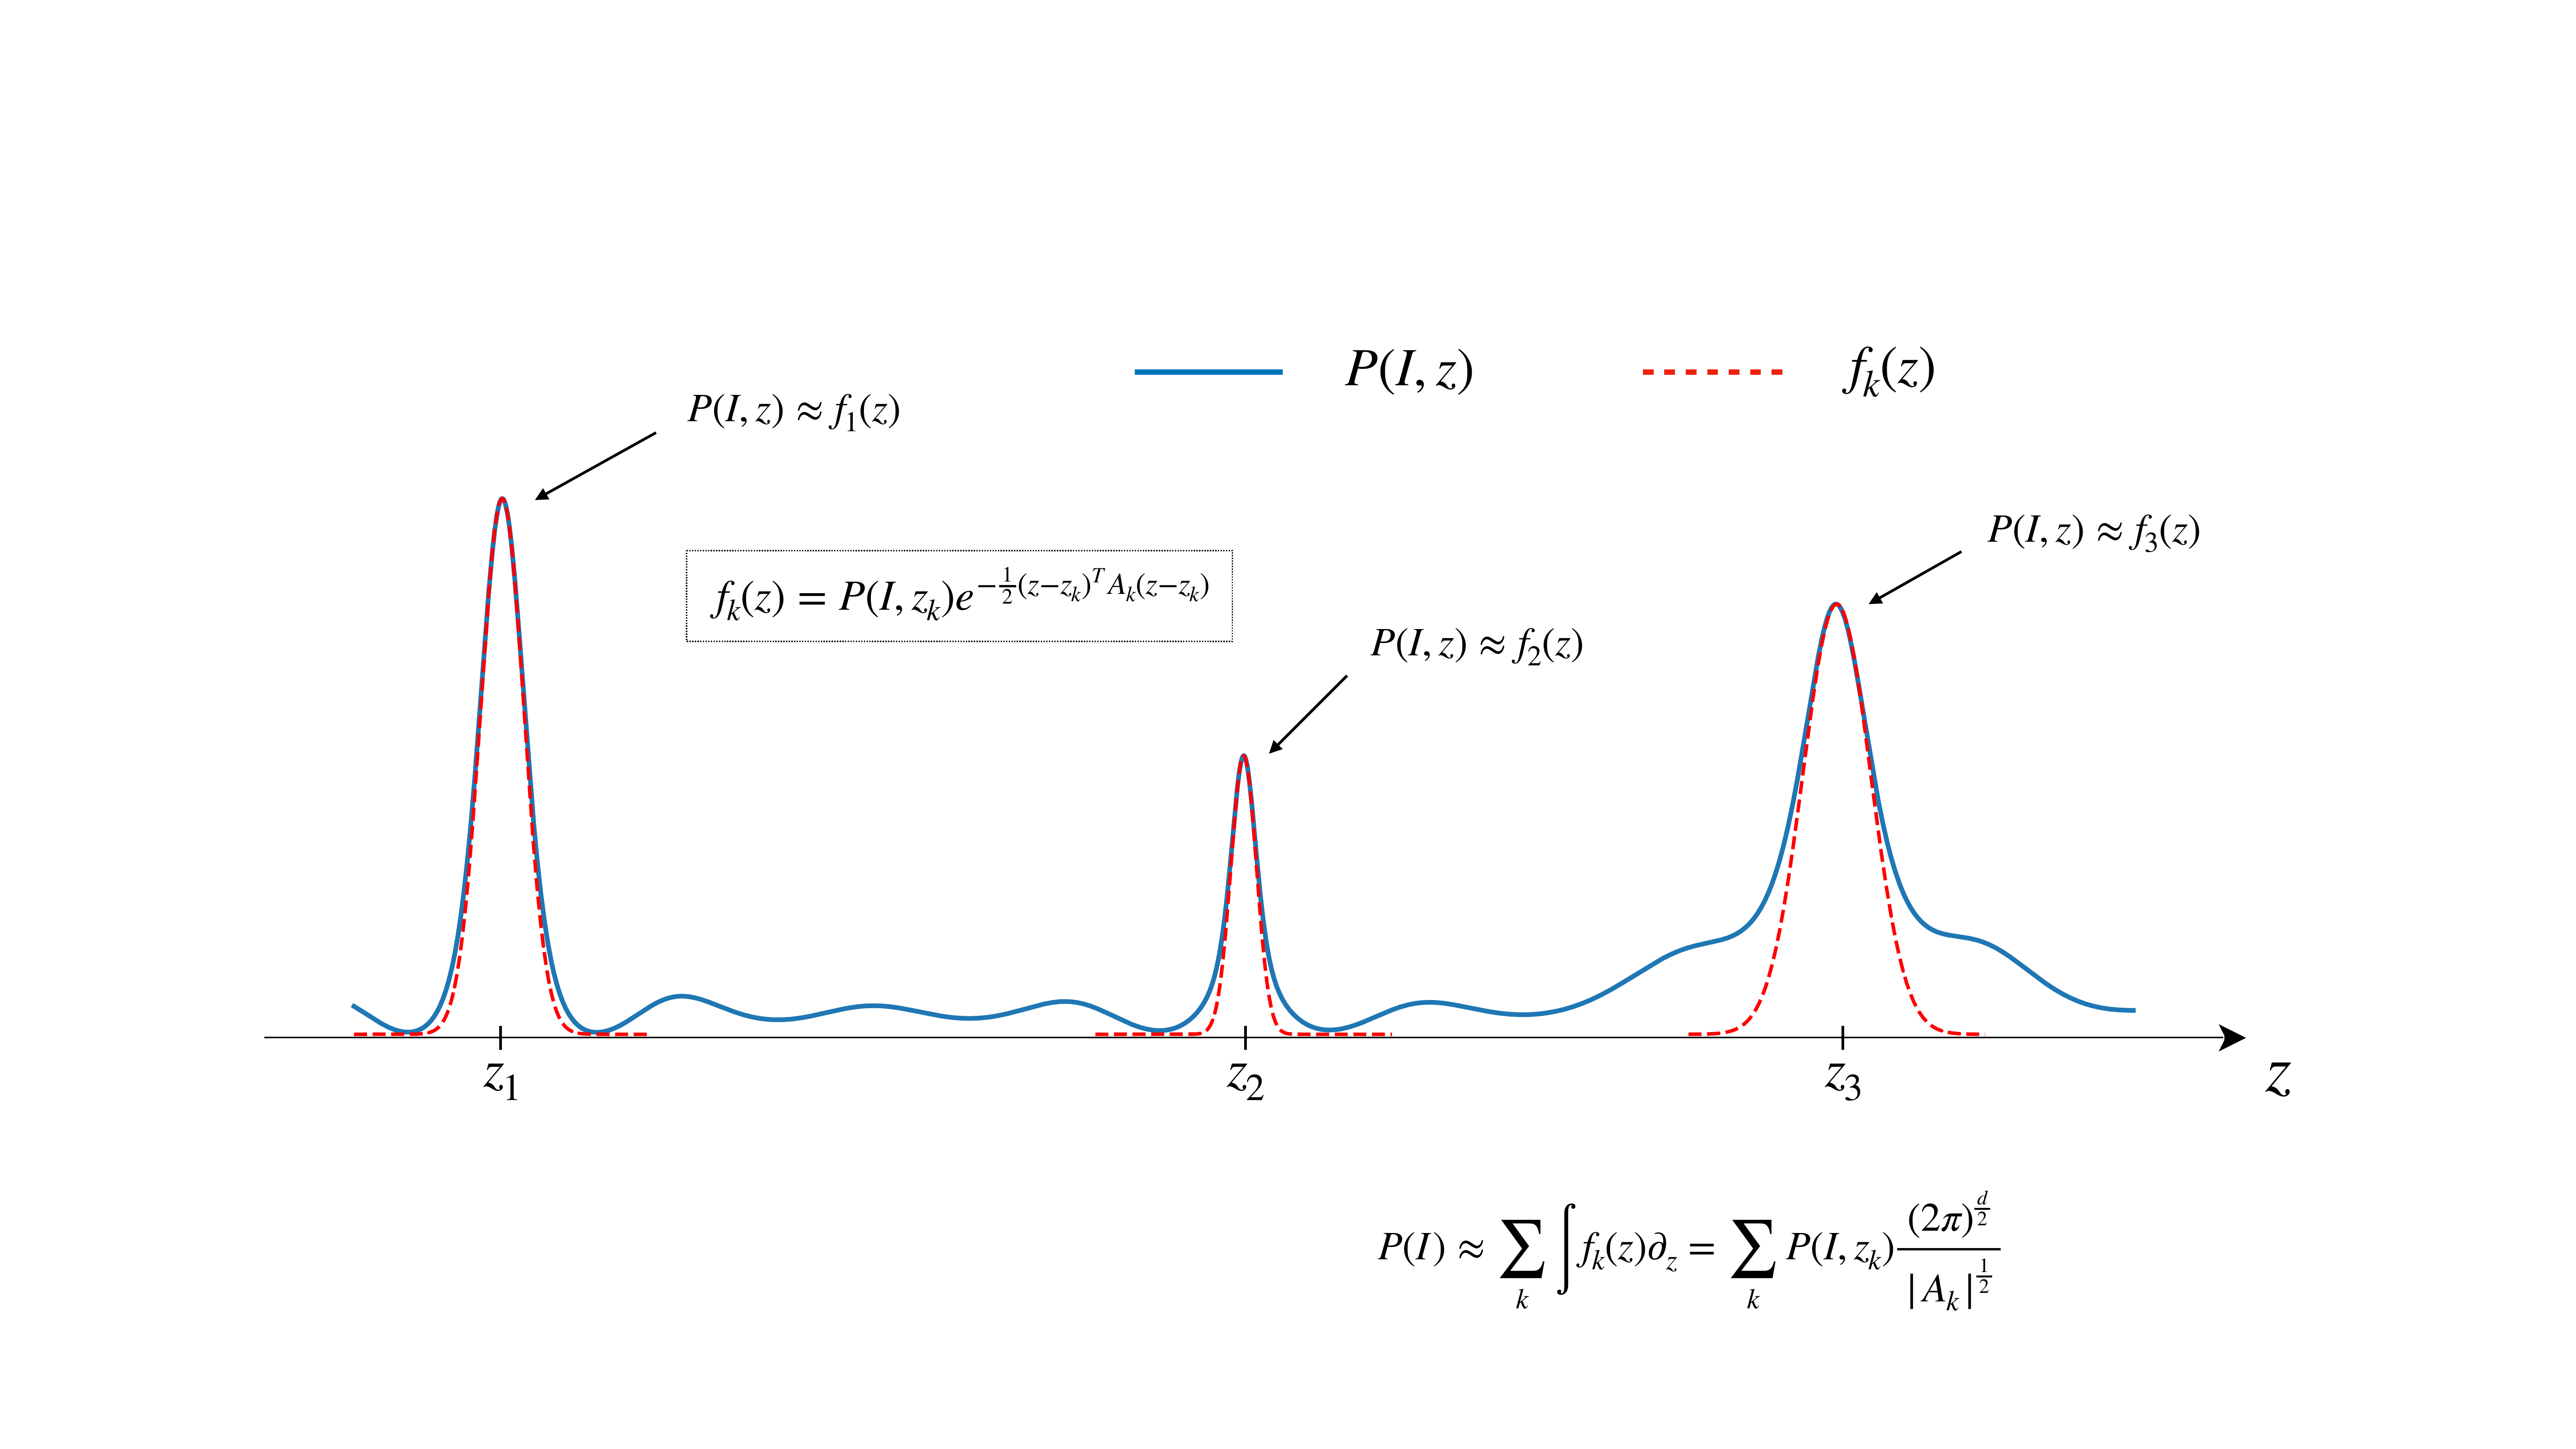}
	\caption{Approximating $P(I,z)$ with Laplace's method for tractable integration.}
    \label{fig:marginals_theory}
\end{figure}
